# Supplementary material for: Search for rare decays of $D^0$ mesons into two muons
Source: arXiv:2212.11203 source file (2023-11-14)
Supplement: Supplementary file 1 [file appendix.tex]

%{\noindent\normalfont\bfseries\Large Appendices}
\section*{Appendices}

\appendix

\section{Appendix}
\label{sec:StandardReferences}
